# Supplementary material for: Pixel Aligned Language Models
Source: arXiv:2312.09237 source file (2023-12-14)
Supplement: Supplementary file 1 [file main_supp.tex]

\documentclass[10pt,twocolumn,letterpaper]{article}

\usepackage[review]{cvpr}      %

\usepackage{graphicx}
\usepackage{amsmath}
\usepackage{amssymb}
\usepackage{pifont} %
\usepackage{enumitem}
\usepackage{booktabs}
\usepackage{setspace}

\input{preamble}

\definecolor{cvprblue}{rgb}{0.21,0.49,0.74}
\usepackage[pagebackref,breaklinks,colorlinks,citecolor=cvprblue]{hyperref}

\newlength\savewidth

\title{Supplementary to Pixel Aligned Language Models}

\author{First Author\\
Institution1\\
Institution1 address\\
{\tt\small firstauthor@i1.org}
\and
Second Author\\
Institution2\\
First line of institution2 address\\
{\tt\small secondauthor@i2.org}
}

\begin{document}
\maketitle

\input{sec/6_supplement.tex}
\vspace{-2mm}
\begin{spacing}{0.8}
{
    \footnotesize
    \bibliographystyle{ieeenat_fullname}
    \bibliography{main}
}
\end{spacing}
\end{document}
